# Supplementary material for: Network Centrality as a New Perspective on Microservice Architecture
Source: arXiv:2501.13520 source file (2025-01-23)
Supplement: Supplementary file 1 [file appendix_main.tex]

\setcounter{table}{0}
\begin{landscape}
\begin{table}[]
\caption{Analyzed Java Spring Microservice OSS Projects}
\label{tab:dataset}
\begin{tabular}{l|ccccc|ccc|cccc}
\multicolumn{1}{c|}{GitHub Project}                                              & \multicolumn{5}{c}{Repository statistics}        & \multicolumn{3}{|c|}{Code2DFD}                                                                    & \multicolumn{4}{c}{Academic Source}                                                                                                                      \\
User/Repository                                             & \multicolumn{1}{l}{Releases} & \multicolumn{1}{l}{Commits} & \multicolumn{1}{l}{Stars} & \multicolumn{1}{l}{PRs open} & \multicolumn{1}{l|}{PRs closed} & \multicolumn{1}{l}{Components} & \multicolumn{1}{l}{Connections} & \multicolumn{1}{l|}{External} & Imranur  & Schneider  & Yang  & Amoroso  \\ \hline
ammiladi/geocoder-microservices                    & 0                            & 24                          & 5                         & 0                            & 0                               & 8                              & 18                              & 1                             &                                              &                    & x                                      &                                             \\
anilallewar/microservices-basics-spring-boot       & 0                            & 46                          & 722                       & 2                            & 6                               & 11                             & 18                              & 2                             &                                              & x                  &                                        &                                             \\
apssouza22/java-microservice                       & 0                            & 140                         & 393                       & 6                            & 6                               & 13                             & 37                              & 2                             &                                              & x                  &                                        &                                             \\
callistaenterprise/blog-microservices              & 14                           & 181                         & 406                       & 0                            & 1                               & 16                             & 19                              & 1                             &                                              & x                  &                                        &                                             \\
dice-group/Basilisk                                & 0                            & 227                         & 2                         & 1                            & 7                               & 4                              & 6                               & 2                             &                                              &                    &                                        & x                                           \\
digital-thinking/micro\_webshop                    & 0                            & 47                          & 1                         & 0                            & 0                               & 8                              & 15                              & 4                             &                                              &                    & x                                      &                                             \\
ewolff/microservice                                & 0                            & 140                         & 725                       & 1                            & 12                              & 6                              & 13                              & 1                             & x                                            & x                  &                                        &                                             \\
ewolff/microservice-consul                         & 0                            & 88                          & 106                       & 1                            & 6                               & 6                              & 12                              & 1                             & x                                            &                    &                                        &                                             \\
ewolff/microservice-kafka                          & 0                            & 101                         & 585                       & 2                            & 8                               & 7                              & 15                              & 1                             &                                              & x                  &                                        &                                             \\
Fatezhang/scaffold-cloud                           & 0                            & 170                         & 89                        & 6                            & 8                               & 19                             & 13                              & 1                             &                                              &                    &                                        & x                                           \\
fernandoabcampos/spring-netflix-oss-microservices  & 0                            & 90                          & 13                        & 0                            & 0                               & 9                              & 20                              & 2                             & x                                            & x                  &                                        &                                             \\
flowant/website                                    & 0                            & 302                         & 1                         & 30                           & 12                              & 6                              & 7                               & 1                             &                                              &                    &                                        & x                                           \\
FudanSELab/train-ticket                            & 7                            & 323                         & 716                       & 4                            & 121                             & 70                             & 113                             & 27                            &                                              &                    & x                                      & x                                           \\
jferrater/Tap-And-Eat-MicroServices                & 0                            & 35                          & 8                         & 0                            & 0                               & 8                              & 16                              & 1                             & x                                            & x                  &                                        &                                             \\
JoeCao/qbike                                       & 1                            & 62                          & 507                       & 2                            & 1                               & 10                             & 23                              & 5                             & x                                            &                    &                                        &                                             \\
koushikkothagal/spring-boot-microservices-workshop & 0                            & 12                          & 740                       & 5                            & 5                               & 4                              & 5                               & 0                             &                                              & x                  &                                        &                                             \\
mdeket/spring-cloud-movie-recommendation           & 0                            & 6                           & 18                        & 0                            & 0                               & 6                              & 15                              & 2                             &                                              & x                  &                                        &                                             \\
novelvast/DentalAppointment                        & 0                            & 92                          & 4                         & 0                            & 0                               & 8                              & 17                              & 7                             &                                              &                    & x                                      &                                             \\
oktadeveloper/jhipster-microservices-example       & 0                            & 76                          & 126                       & 3                            & 61                              & 6                              & 9                               & 2                             &                                              &                    &                                        & x                                           \\
piomin/sample-spring-cloud-webflux                 & 0                            & 126                         & 98                        & 0                            & 102                             & 4                              & 7                               & 1                             &                                              &                    & x                                      &                                             \\
piomin/sample-spring-microservices-new             & 0                            & 179                         & 1184                      & 0                            & 116                             & 7                              & 21                              & 1                             &                                              &                    & x                                      & x                                           \\
rohitghatol/spring-boot-microservices              & 0                            & 66                          & 1773                      & 2                            & 9                               & 8                              & 17                              & 2                             &                                              & x                  &                                        &                                             \\
sqshq/piggymetrics                                 & 2                            & 290                         & 13256                     & 12                           & 45                              & 14                             & 34                              & 3                             &                                              & x                  & x                                      &                                             \\
umarafzl/springcloudmicroservices                  & 0                            & 1                           & 0                         & 0                            & 0                               & 5                              & 12                              & 3                             &                                              &                    & x                                      &                                            
\end{tabular}
\end{table}
\end{landscape}
\setcounter{table}{1}
\begin{landscape}
\begin{table}[]
\centering
\caption{Metrics extracted from Understand and applied aggregation methods}
\begin{tabular}{l|l|l|l|l|l}
Short name                & Full name                        & Type & Sum() aggregation & Max() aggregation & Avg() aggregation \\ \hline
CountDeclFile             & Number of Files                  & Size & x                 & -                 & -                 \\
CountLine                 & Number of Lines                  & Size & x                 & -                 & -                 \\
CountLineBlank            & Blank Lines of Code              & Size & x                 & -                 & -                 \\
CountLineCode             & Lines of Code                    & Size & x                 & -                 & -                 \\
CountLineComment          & Comment Lines                    & Size & x                 & -                 & -                 \\
CountStmt                 & Number of Statements             & Size & x                 & -                 & -                 \\
CountStmtDecl             & Number of Declarative Statements & Size & x                 & -                 & -                 \\
CountStmtExe              & Number of Executable Statements  & Size & x                 & -                 & -                 \\
CountDeclClass            & Number of Classes                & Size & x                 & -                 & -                 \\
CountDeclClassMethod      & Number of Class Methods          & Size & x                 & -                 & -                 \\
CountDeclClassVariable    & Number of Class Variables        & Size & x                 & -                 & -                 \\
CountDeclFunction         & Number of Functions              & Size & x                 & -                 & -                 \\
CountDeclInstanceMethod   & Number of Instance Methods       & Size & x                 & -                 & -                 \\
CountDeclInstanceVariable & Number of Instance Variables     & Size & x                 & -                 & -                 \\
CountDeclMethod           & Number of Methods                & Size & x                 & -                 & -                 \\
CountDeclMethodDefault    & Number of Default Methods        & Size & x                 & -                 & -                 \\
CountDeclMethodPrivate    & Number of Private Methods        & Size & x                 & -                 & -                 \\
CountDeclMethodProtected  & Number of Protected Methods      & Size & x                 & -                 & -                 \\
CountDeclMethodPublic     & Number of Public Methods         & Size & x                 & -                 & -                 \\
CountLineCodeDecl         & Number of Declarative Code Lines & Size & x                 & -                 & -                 \\
CountLineCodeExe          & Number of Executable Code Lines  & Size & x                 & -                 & -                 \\
CountSemicolon            & Number of Semicolons             & Size & x                 & -                 & -                \\
SumCyclomatic            & Sum of Cyclomatic Complexity             & Complexity & x                 & -                 & -                
\end{tabular}
\end{table}
\end{landscape}
\setcounter{table}{2}
\begin{landscape}
\begin{table}[]
\centering
\caption{Metrics extracted from Jasome and applied aggregation methods}
\begin{tabular}{l|l|l|l|l|l}
Short name & Full name                              & Type       & Sum() aggregation & Max() aggregation & Avg() aggregation \\ \hline
TLOC       & Total Lines of Code                    & Size       & x                 & -                 & -                 \\
RTLOC      & Raw Total Lines of Code                & Size       & x                 & -                 & -                 \\
NF         & Number of Attributes                   & Size       & x                 & -                 & x                 \\
NSF        & Number of Static Attributes            & Size       & x                 & -                 & x                 \\
NPF        & Number of Public Attributes            & Size       & x                 & -                 & x                 \\
NM         & Number of Methods                      & Size       & x                 & -                 & x                 \\
NSM        & Number of Static Methods               & Size       & x                 & -                 & x                 \\
NPM        & Number of Public Methods               & Size       & x                 & -                 & x                 \\
NOC        & Number of Classes                      & Size       & x                 & -                 & -                 \\
DIT        & Depth of Inheritance Tree              & Complexity & -                 & x                 & x                 \\
NORM       & Number of Overridden Methods           & Complexity & x                 & -                 & x                 \\
NMI        & Number of Inherited Methods            & Complexity & x                 & -                 & x                 \\
NMA        & Number of Methods Added to Inheritance & Complexity & x                 & -                 & x                 \\
SIX        & Specialization Index                   & Complexity & x                 & -                 & x                 \\
Mit        & Number of Methods Inherited Total      & Complexity & x                 & -                 & x                 \\
Mi         & Number of Methods Inherited            & Complexity & x                 & -                 & x                 \\
Md         & Number of Methods Defined              & Complexity & x                 & -                 & x                 \\
Mo         & Number of Methods Overidden            & Complexity & x                 & -                 & x                 \\
Ma         & Number of Methods (All)                & Complexity & x                 & -                 & x                 \\
MIF        & Method Inheritance Factor              & Complexity & -                 & -                 & x                 \\
PMd        & Number of Public Methods Defined       & Size       & x                 & -                 & x                 \\
PMi        & Number of Public Methods Inherited     & Size       & x                 & -                 & x                 \\
PMR        & Public Methods Ratio                   & Size       & -                 & -                 & x                 \\
HMd        & Number of Hidden Methods Defined       & Size       & x                 & -                 & x                 \\
HMi        & Number of Hidden Methods Inherited     & Size       & x                 & -                 & x                 \\
MHF        & Method Hiding Factor                   & Complexity & -                 & -                 & x                 \\
PF         & Polymorphism Factor                    & Complexity & x                 & -                 & -                 \\
Ait        & Number of Attributes Inherited Total   & Complexity & x                 & -                 & x                 \\
Ad         & Number of Attributes Defined           & Complexity & x                 & -                 & x                 \\
Ao         & Number of Attributes Overidden         & Complexity & x                 & -                 & x                 \\
Aa         & Number of Attributes (All)             & Size       & x                 & -                 & x                 \\
AIF        & Attribute Inheritance Factor           & Complexity & -                 & -                 & x                 \\
Av         & Number of Public Attributes Defined    & Size       & x                 & -                 & x                 \\
AHF        & Attribute Hiding Factor                & Complexity & -                 & -                 & x                 \\
VG         & McCabe Cyclomatic Complexity           & Complexity & x                 & x                 & x                 \\
WMC        & Weighed Methods per Class              & Complexity & x                 & x                 & -                 \\
LCOM       & Lack of Cohesion Methods               & Complexity & x                 & x                 & x                 \\
NOI        & Number of Interfaces                   & Complexity & x                 & -                 & -                 \\
Ca         & Afferent Coupling                      & Complexity & x                 & -                 & -                 \\
Ce         & Efferent Coupling                      & Complexity & x                 & -                 & -                 \\
NBD        & Nested Block Depth                     & Complexity & x                 & x                 & x                 \\
NOCh       & Number of Children                     & Complexity & x                 & -                 & x                 \\
NOPa       & Number of Parents                      & Complexity & x                 & -                 & x                 \\
NOD        & Number of Descendants                  & Complexity & x                 & -                 & x                 \\
NOA        & Number of Ancestors                    & Complexity & x                 & -                 & x                 \\
NOL        & Number of Links                        & Complexity & x                 & -                 & x                 \\
MCLC       & McClure’s Complexity Metric            & Complexity & x                 & x                 & x                 \\
Fout       & Fan-out                                & Complexity & x                 & x                 & x                 \\
Fin        & Fan-in                                 & Complexity & x                 & x                 & x                 \\
Si         & Structural Complexity                  & Complexity & x                 & x                 & x                 \\
IOVars     & Input/Output Variables                 & Complexity & x                 & x                 & x                 \\
Di         & Data Complexity                        & Complexity & x                 & x                 & x                 \\
PkgTCi     & Package Total System Complexity        & Complexity & x                 & -                 & -                 \\
PkgRCi     & Package Relative System Complexity     & Complexity & x                 & -                 & -                
\end{tabular}
\end{table}
\end{landscape}
\setcounter{table}{3}
\begin{landscape}
\begin{table}[]
\centering
\caption{Metrics extracted from SonarQube and applied aggregation methods}
\begin{tabular}{l|l|l|l|l|l}
Short name            & Full name                                           & Type       & Sum() aggregation & Max() aggregation & Avg() aggregation \\ \hline
-                     & Sqale rating (Avg, Max)                             & Quality    & -                 & x                 & x                 \\
-                     & Reliablity rating (Avg, Max)                        & Quality    & -                 & x                 & x                 \\
-                     & Security rating (Avg, Max)                          & Quality    & -                 & x                 & x                 \\
Reliability RE        & Reliability remediation effort                      & Quality    & x                 & -                 & -                 \\
Security RE           & Security remediation effort                         & Quality    & x                 & -                 & -                 \\
SQ Maintainability RE & Software quality maintainability remediation effort & Quality    & x                 & -                 & -                 \\
SQ Reliability RE     & Software quality reliability remediation effort     & Quality    & x                 & -                 & -                 \\
SQ Security RE        & Software quality security remediation effort        & Quality    & x                 & -                 & -                 \\
-                     & Bugs                                                & Quality    & x                 & -                 & -                 \\
-                     & Code smells                                         & Quality    & x                 & -                 & -                 \\
-                     & Violations                                          & Quality    & x                 & -                 & -                 \\
-                     & Critical violations                                 & Quality    & x                 & -                 & -                 \\
-                     & Info violations                                     & Quality    & x                 & -                 & -                 \\
-                     & Major violations                                    & Quality    & x                 & -                 & -                 \\
-                     & Minor violations                                    & Quality    & x                 & -                 & -                 \\
-                     & Duplicated blocks                                   & Quality    & x                 & -                 & -                 \\
-                     & Security hotspots                                   & Quality    & x                 & -                 & -                 \\
-                     & Effort to reach quality rating A                    & Quality    & x                 & -                 & -                 \\
-                     & Cognitive complexity                                & Complexity & x                 & -                 & -                 
\end{tabular}
\end{table}
\end{landscape}
