# Supplementary material for: Network Centrality as a New Perspective on Microservice Architecture
Source: arXiv:2501.13520 source file (2025-01-23)
Supplement: Supplementary file 2 [file dataset.tex]

\setcounter{table}{0}
\begin{landscape}
\begin{table}[]
\caption{Analyzed Java Spring Microservice OSS Projects}
\label{tab:dataset}
\begin{tabular}{l|ccccc|ccc|cccc}
\multicolumn{1}{c|}{GitHub Project}                                              & \multicolumn{5}{c}{Repository statistics}        & \multicolumn{3}{|c|}{Code2DFD}                                                                    & \multicolumn{4}{c}{Academic Source}                                                                                                                      \\
User/Repository                                             & \multicolumn{1}{l}{Releases} & \multicolumn{1}{l}{Commits} & \multicolumn{1}{l}{Stars} & \multicolumn{1}{l}{PRs open} & \multicolumn{1}{l|}{PRs closed} & \multicolumn{1}{l}{Components} & \multicolumn{1}{l}{Connections} & \multicolumn{1}{l|}{External} & Imranur  & Schneider  & Yang  & Amoroso  \\ \hline
ammiladi/geocoder-microservices                    & 0                            & 24                          & 5                         & 0                            & 0                               & 8                              & 18                              & 1                             &                                              &                    & x                                      &                                             \\
anilallewar/microservices-basics-spring-boot       & 0                            & 46                          & 722                       & 2                            & 6                               & 11                             & 18                              & 2                             &                                              & x                  &                                        &                                             \\
apssouza22/java-microservice                       & 0                            & 140                         & 393                       & 6                            & 6                               & 13                             & 37                              & 2                             &                                              & x                  &                                        &                                             \\
callistaenterprise/blog-microservices              & 14                           & 181                         & 406                       & 0                            & 1                               & 16                             & 19                              & 1                             &                                              & x                  &                                        &                                             \\
dice-group/Basilisk                                & 0                            & 227                         & 2                         & 1                            & 7                               & 4                              & 6                               & 2                             &                                              &                    &                                        & x                                           \\
digital-thinking/micro\_webshop                    & 0                            & 47                          & 1                         & 0                            & 0                               & 8                              & 15                              & 4                             &                                              &                    & x                                      &                                             \\
ewolff/microservice                                & 0                            & 140                         & 725                       & 1                            & 12                              & 6                              & 13                              & 1                             & x                                            & x                  &                                        &                                             \\
ewolff/microservice-consul                         & 0                            & 88                          & 106                       & 1                            & 6                               & 6                              & 12                              & 1                             & x                                            &                    &                                        &                                             \\
ewolff/microservice-kafka                          & 0                            & 101                         & 585                       & 2                            & 8                               & 7                              & 15                              & 1                             &                                              & x                  &                                        &                                             \\
Fatezhang/scaffold-cloud                           & 0                            & 170                         & 89                        & 6                            & 8                               & 19                             & 13                              & 1                             &                                              &                    &                                        & x                                           \\
fernandoabcampos/spring-netflix-oss-microservices  & 0                            & 90                          & 13                        & 0                            & 0                               & 9                              & 20                              & 2                             & x                                            & x                  &                                        &                                             \\
flowant/website                                    & 0                            & 302                         & 1                         & 30                           & 12                              & 6                              & 7                               & 1                             &                                              &                    &                                        & x                                           \\
FudanSELab/train-ticket                            & 7                            & 323                         & 716                       & 4                            & 121                             & 70                             & 113                             & 27                            &                                              &                    & x                                      & x                                           \\
jferrater/Tap-And-Eat-MicroServices                & 0                            & 35                          & 8                         & 0                            & 0                               & 8                              & 16                              & 1                             & x                                            & x                  &                                        &                                             \\
JoeCao/qbike                                       & 1                            & 62                          & 507                       & 2                            & 1                               & 10                             & 23                              & 5                             & x                                            &                    &                                        &                                             \\
koushikkothagal/spring-boot-microservices-workshop & 0                            & 12                          & 740                       & 5                            & 5                               & 4                              & 5                               & 0                             &                                              & x                  &                                        &                                             \\
mdeket/spring-cloud-movie-recommendation           & 0                            & 6                           & 18                        & 0                            & 0                               & 6                              & 15                              & 2                             &                                              & x                  &                                        &                                             \\
novelvast/DentalAppointment                        & 0                            & 92                          & 4                         & 0                            & 0                               & 8                              & 17                              & 7                             &                                              &                    & x                                      &                                             \\
oktadeveloper/jhipster-microservices-example       & 0                            & 76                          & 126                       & 3                            & 61                              & 6                              & 9                               & 2                             &                                              &                    &                                        & x                                           \\
piomin/sample-spring-cloud-webflux                 & 0                            & 126                         & 98                        & 0                            & 102                             & 4                              & 7                               & 1                             &                                              &                    & x                                      &                                             \\
piomin/sample-spring-microservices-new             & 0                            & 179                         & 1184                      & 0                            & 116                             & 7                              & 21                              & 1                             &                                              &                    & x                                      & x                                           \\
rohitghatol/spring-boot-microservices              & 0                            & 66                          & 1773                      & 2                            & 9                               & 8                              & 17                              & 2                             &                                              & x                  &                                        &                                             \\
sqshq/piggymetrics                                 & 2                            & 290                         & 13256                     & 12                           & 45                              & 14                             & 34                              & 3                             &                                              & x                  & x                                      &                                             \\
umarafzl/springcloudmicroservices                  & 0                            & 1                           & 0                         & 0                            & 0                               & 5                              & 12                              & 3                             &                                              &                    & x                                      &                                            
\end{tabular}
\end{table}
\end{landscape}
