# Supplementary material for: Network Centrality as a New Perspective on Microservice Architecture
Source: arXiv:2501.13520 source file (2025-01-23)
Supplement: Supplementary file 3 [file jasome.tex]

\setcounter{table}{2}
\begin{landscape}
\begin{table}[]
\centering
\caption{Metrics extracted from Jasome and applied aggregation methods}
\begin{tabular}{l|l|l|l|l|l}
Short name & Full name                              & Type       & Sum() aggregation & Max() aggregation & Avg() aggregation \\ \hline
TLOC       & Total Lines of Code                    & Size       & x                 & -                 & -                 \\
RTLOC      & Raw Total Lines of Code                & Size       & x                 & -                 & -                 \\
NF         & Number of Attributes                   & Size       & x                 & -                 & x                 \\
NSF        & Number of Static Attributes            & Size       & x                 & -                 & x                 \\
NPF        & Number of Public Attributes            & Size       & x                 & -                 & x                 \\
NM         & Number of Methods                      & Size       & x                 & -                 & x                 \\
NSM        & Number of Static Methods               & Size       & x                 & -                 & x                 \\
NPM        & Number of Public Methods               & Size       & x                 & -                 & x                 \\
NOC        & Number of Classes                      & Size       & x                 & -                 & -                 \\
DIT        & Depth of Inheritance Tree              & Complexity & -                 & x                 & x                 \\
NORM       & Number of Overridden Methods           & Complexity & x                 & -                 & x                 \\
NMI        & Number of Inherited Methods            & Complexity & x                 & -                 & x                 \\
NMA        & Number of Methods Added to Inheritance & Complexity & x                 & -                 & x                 \\
SIX        & Specialization Index                   & Complexity & x                 & -                 & x                 \\
Mit        & Number of Methods Inherited Total      & Complexity & x                 & -                 & x                 \\
Mi         & Number of Methods Inherited            & Complexity & x                 & -                 & x                 \\
Md         & Number of Methods Defined              & Complexity & x                 & -                 & x                 \\
Mo         & Number of Methods Overidden            & Complexity & x                 & -                 & x                 \\
Ma         & Number of Methods (All)                & Complexity & x                 & -                 & x                 \\
MIF        & Method Inheritance Factor              & Complexity & -                 & -                 & x                 \\
PMd        & Number of Public Methods Defined       & Size       & x                 & -                 & x                 \\
PMi        & Number of Public Methods Inherited     & Size       & x                 & -                 & x                 \\
PMR        & Public Methods Ratio                   & Size       & -                 & -                 & x                 \\
HMd        & Number of Hidden Methods Defined       & Size       & x                 & -                 & x                 \\
HMi        & Number of Hidden Methods Inherited     & Size       & x                 & -                 & x                 \\
MHF        & Method Hiding Factor                   & Complexity & -                 & -                 & x                 \\
PF         & Polymorphism Factor                    & Complexity & x                 & -                 & -                 \\
Ait        & Number of Attributes Inherited Total   & Complexity & x                 & -                 & x                 \\
Ad         & Number of Attributes Defined           & Complexity & x                 & -                 & x                 \\
Ao         & Number of Attributes Overidden         & Complexity & x                 & -                 & x                 \\
Aa         & Number of Attributes (All)             & Size       & x                 & -                 & x                 \\
AIF        & Attribute Inheritance Factor           & Complexity & -                 & -                 & x                 \\
Av         & Number of Public Attributes Defined    & Size       & x                 & -                 & x                 \\
AHF        & Attribute Hiding Factor                & Complexity & -                 & -                 & x                 \\
VG         & McCabe Cyclomatic Complexity           & Complexity & x                 & x                 & x                 \\
WMC        & Weighed Methods per Class              & Complexity & x                 & x                 & -                 \\
LCOM       & Lack of Cohesion Methods               & Complexity & x                 & x                 & x                 \\
NOI        & Number of Interfaces                   & Complexity & x                 & -                 & -                 \\
Ca         & Afferent Coupling                      & Complexity & x                 & -                 & -                 \\
Ce         & Efferent Coupling                      & Complexity & x                 & -                 & -                 \\
NBD        & Nested Block Depth                     & Complexity & x                 & x                 & x                 \\
NOCh       & Number of Children                     & Complexity & x                 & -                 & x                 \\
NOPa       & Number of Parents                      & Complexity & x                 & -                 & x                 \\
NOD        & Number of Descendants                  & Complexity & x                 & -                 & x                 \\
NOA        & Number of Ancestors                    & Complexity & x                 & -                 & x                 \\
NOL        & Number of Links                        & Complexity & x                 & -                 & x                 \\
MCLC       & McClure’s Complexity Metric            & Complexity & x                 & x                 & x                 \\
Fout       & Fan-out                                & Complexity & x                 & x                 & x                 \\
Fin        & Fan-in                                 & Complexity & x                 & x                 & x                 \\
Si         & Structural Complexity                  & Complexity & x                 & x                 & x                 \\
IOVars     & Input/Output Variables                 & Complexity & x                 & x                 & x                 \\
Di         & Data Complexity                        & Complexity & x                 & x                 & x                 \\
PkgTCi     & Package Total System Complexity        & Complexity & x                 & -                 & -                 \\
PkgRCi     & Package Relative System Complexity     & Complexity & x                 & -                 & -                
\end{tabular}
\end{table}
\end{landscape}
