# Supplementary material for: Network Centrality as a New Perspective on Microservice Architecture
Source: arXiv:2501.13520 source file (2025-01-23)
Supplement: Supplementary file 4 [file sonarqube.tex]

\setcounter{table}{3}
\begin{landscape}
\begin{table}[]
\centering
\caption{Metrics extracted from SonarQube and applied aggregation methods}
\begin{tabular}{l|l|l|l|l|l}
Short name            & Full name                                           & Type       & Sum() aggregation & Max() aggregation & Avg() aggregation \\ \hline
-                     & Sqale rating (Avg, Max)                             & Quality    & -                 & x                 & x                 \\
-                     & Reliablity rating (Avg, Max)                        & Quality    & -                 & x                 & x                 \\
-                     & Security rating (Avg, Max)                          & Quality    & -                 & x                 & x                 \\
Reliability RE        & Reliability remediation effort                      & Quality    & x                 & -                 & -                 \\
Security RE           & Security remediation effort                         & Quality    & x                 & -                 & -                 \\
SQ Maintainability RE & Software quality maintainability remediation effort & Quality    & x                 & -                 & -                 \\
SQ Reliability RE     & Software quality reliability remediation effort     & Quality    & x                 & -                 & -                 \\
SQ Security RE        & Software quality security remediation effort        & Quality    & x                 & -                 & -                 \\
-                     & Bugs                                                & Quality    & x                 & -                 & -                 \\
-                     & Code smells                                         & Quality    & x                 & -                 & -                 \\
-                     & Violations                                          & Quality    & x                 & -                 & -                 \\
-                     & Critical violations                                 & Quality    & x                 & -                 & -                 \\
-                     & Info violations                                     & Quality    & x                 & -                 & -                 \\
-                     & Major violations                                    & Quality    & x                 & -                 & -                 \\
-                     & Minor violations                                    & Quality    & x                 & -                 & -                 \\
-                     & Duplicated blocks                                   & Quality    & x                 & -                 & -                 \\
-                     & Security hotspots                                   & Quality    & x                 & -                 & -                 \\
-                     & Effort to reach quality rating A                    & Quality    & x                 & -                 & -                 \\
-                     & Cognitive complexity                                & Complexity & x                 & -                 & -                 
\end{tabular}
\end{table}
\end{landscape}
