# Supplementary material for: Network Centrality as a New Perspective on Microservice Architecture
Source: arXiv:2501.13520 source file (2025-01-23)
Supplement: Supplementary file 5 [file understand.tex]

\setcounter{table}{1}
\begin{landscape}
\begin{table}[]
\centering
\caption{Metrics extracted from Understand and applied aggregation methods}
\begin{tabular}{l|l|l|l|l|l}
Short name                & Full name                        & Type & Sum() aggregation & Max() aggregation & Avg() aggregation \\ \hline
CountDeclFile             & Number of Files                  & Size & x                 & -                 & -                 \\
CountLine                 & Number of Lines                  & Size & x                 & -                 & -                 \\
CountLineBlank            & Blank Lines of Code              & Size & x                 & -                 & -                 \\
CountLineCode             & Lines of Code                    & Size & x                 & -                 & -                 \\
CountLineComment          & Comment Lines                    & Size & x                 & -                 & -                 \\
CountStmt                 & Number of Statements             & Size & x                 & -                 & -                 \\
CountStmtDecl             & Number of Declarative Statements & Size & x                 & -                 & -                 \\
CountStmtExe              & Number of Executable Statements  & Size & x                 & -                 & -                 \\
CountDeclClass            & Number of Classes                & Size & x                 & -                 & -                 \\
CountDeclClassMethod      & Number of Class Methods          & Size & x                 & -                 & -                 \\
CountDeclClassVariable    & Number of Class Variables        & Size & x                 & -                 & -                 \\
CountDeclFunction         & Number of Functions              & Size & x                 & -                 & -                 \\
CountDeclInstanceMethod   & Number of Instance Methods       & Size & x                 & -                 & -                 \\
CountDeclInstanceVariable & Number of Instance Variables     & Size & x                 & -                 & -                 \\
CountDeclMethod           & Number of Methods                & Size & x                 & -                 & -                 \\
CountDeclMethodDefault    & Number of Default Methods        & Size & x                 & -                 & -                 \\
CountDeclMethodPrivate    & Number of Private Methods        & Size & x                 & -                 & -                 \\
CountDeclMethodProtected  & Number of Protected Methods      & Size & x                 & -                 & -                 \\
CountDeclMethodPublic     & Number of Public Methods         & Size & x                 & -                 & -                 \\
CountLineCodeDecl         & Number of Declarative Code Lines & Size & x                 & -                 & -                 \\
CountLineCodeExe          & Number of Executable Code Lines  & Size & x                 & -                 & -                 \\
CountSemicolon            & Number of Semicolons             & Size & x                 & -                 & -                \\
SumCyclomatic            & Sum of Cyclomatic Complexity             & Complexity & x                 & -                 & -                
\end{tabular}
\end{table}
\end{landscape}
